# Supplementary material for: On the Interplay between Self-Driving Cars and Public Transportation
Source: arXiv:2109.01627 source file (2023-12-23)
Supplement: Supplementary file 1 [file appendixcomputation.tex]

\section{Computation of Equilibria}
\label{app:computation}

We compute equilibria via the best-response algorithm. It is well-known that the best-response algorithm has no convergence guarantee. Yet, if it converges, then it converges to an equilibrium. In practice, we implement two versions of the best response algorithm and we stop at a so-called $\varepsilon$-equilibrium, as we detail below.
\begin{description}
\item[Synchronous best response:]
We iteratively compute the players' actions by
\begin{equation*}
\begin{aligned}
    \priceStrategy{1,n+1} &\in\bestResponse{1}(\priceStrategy{2,n}) \\
    \priceStrategy{2,n+1} &\in\bestResponse{2}(\priceStrategy{1,n}),
\end{aligned}
\end{equation*}
and select random $\priceStrategy{j,0}\in\priceStrategiesSet{j}$ for $j\in\{1,2\}$. At the end of each iteration we check the stopping criterion: We stop if both players do not improve their profit more than $\varepsilon$; i.e., if for all $j\in\{1,2\}$ we have
\begin{equation*}
     \frac{\utility_j(\priceStrategy{j,n+1},\{\customersEquilibria{i}(\priceStrategy{j,n+1},\priceStrategy{-j,n})\}_{i=1}^{\demandNumber})
    -
    \utility_j(\priceStrategy{j,n},\{\customersEquilibria{i}(\priceStrategy{j,n},\priceStrategy{-j,n})\}_{i=1}^{\demandNumber})}
    {\utility_j(\priceStrategy{j,n},\{\customersEquilibria{i}(\priceStrategy{j,n},\priceStrategy{-j,n})\}_{i=1}^{\demandNumber})}\leq\varepsilon.
\end{equation*}
Then, $(\priceStrategy{1,n},\priceStrategy{2,n})$ is an $\varepsilon$-equilibrium.

\item[Asynchronous best response:]
We iteratively compute the players' actions by
\begin{equation*}
\begin{aligned}
    \priceStrategy{1,n+1} &\in\bestResponse{1}(\priceStrategy{2,n}) \\
    \priceStrategy{2,n+1} &\in\bestResponse{2}(\priceStrategy{1,n+1}),
\end{aligned}
\end{equation*}
and select random $\priceStrategy{2,0}\in\priceStrategiesSet{2}$.
After the computation of each best-response (and not after each iteration), we check the stopping criterion, again formulated based on the definition $\varepsilon$-equilibrium. In particular, we stop if 
\begin{equation*}
\frac{\utility_1(\priceStrategy{1,n+1},\{\customersEquilibria{i}(\priceStrategy{1,n+1},\priceStrategy{2,n})\}_{i=1}^{\demandNumber})
    -
    \utility_1(\priceStrategy{1,n},\{\customersEquilibria{i}(\priceStrategy{1,n},\priceStrategy{2,n})\}_{i=1}^{\demandNumber})}
    {\utility_1(\priceStrategy{1,n},\{\customersEquilibria{i}(\priceStrategy{1,n},\priceStrategy{2,n})\}_{i=1}^{\demandNumber})}\leq\varepsilon,
\end{equation*}
which yields the $\varepsilon$-equilibrium $(\priceStrategy{1,n},\priceStrategy{2,n})$, or if
\begin{equation*}
\frac{\utility_2(\priceStrategy{2,n},\{\customersEquilibria{i}(\priceStrategy{1,n+1},\priceStrategy{2,n+1})\}_{i=1}^{\demandNumber})
    -
    \utility_2(\priceStrategy{2,n+1},\{\customersEquilibria{i}(\priceStrategy{1,n+1},\priceStrategy{2,n+1})\}_{i=1}^{\demandNumber})}
    {\utility_2(\priceStrategy{2,n},\{\customersEquilibria{i}(\priceStrategy{1,n},\priceStrategy{2,n})\}_{i=1}^{\demandNumber})}\leq\varepsilon,
\end{equation*}
which yields the $\varepsilon$-equilibrium $(\priceStrategy{1,n+1},\priceStrategy{2,n})$.
\end{description}
For our case studies we used both versions and select them based on their empirical performance. For the identical \gls{abk:amod} operators case we used $\varepsilon=\SI{0.01}{\percent}$, for the non-identical \gls{abk:amod} operators case we used $\varepsilon=\SI{0.1}{\percent}$.

The computational time spans from \SIrange{20}{40}{\minute} for the two identical \gls{abk:amod} operator case to up to several hours for the two non-identical \gls{abk:amod} operator case. The degenerate case of a single \gls{abk:amod} operator can be solved in less than one second. 
We implemented our cases studies in Matlab on commodity hardware (\SI{2.3}{\giga\hertz} Quad-core with \SI{16}{\giga\byte} of RAM). We use YALMIP \citep{Lofberg2004} to formulate optimization problems, Gurobi \citep{gurobi} to solve quadratic programs, and Mosek \citep{mosek} to solve second-order conic programs.

Finally, we note that the game will generally have multiple equilibria. Accordingly, we ran the algorithm with different initial conditions, but we never observed the algorithm converging to different equilibria.
